# Supplementary material for: Dynamically Feasible Path Planning in Cluttered Environments via Reachable Bezier Polytopes
Source: arXiv:2411.13507 source file (2024-11-20)
Supplement: Supplementary file 1 [file Appendix.tex]

\section{Appendix}
